# Supplementary material for: Multi-Broadcasting under the SINR Model
Source: arXiv:1504.01352 source file (2015-04-06)
Supplement: Supplementary file 1 [file appendix.tex]

\appendix

\section{Reviewers comments for read made reference}
In multi-broadcasting, k rumors have to be transmitted throughout a network of n nodes concurrently. The paper proposes algorithms for multi-broadcasting when nodes are embedded in the 2D plane and transmit according to the signal-to-interference-plus-noise ratio (SINR). Every transmitting node is assumed to access the wireless medium at unit power, and in a single round it can transmit a single rumor plus O(log N) control bits (where N is the size of the ID space).

Algorithms are based on a graph structure for a suitable definition of neighborhood based on SINR reception. The running times depend on parameters like the diameter D or maximum degree $\Delta$. The paper proposes algorithms under different informational assumptions, where nodes - in addition to $n,N,k,D,\Delta$ - know (1) the entire network with coordinates, (2) only their coordinates and the ones of their neighbors, (3) only their own coordinates, and (4) only their own label and the label of their neighbors. The running times are roughly (D+k)*polylog(n) for (1) and (2), and roughly $(n+k)\lg n$ for (3) and (4).

The general idea is sectioning the plane, elect a leader in each box, build a backbone structure (like a connected dominating set), collect and broadcast the rumors. This scheme seems quite similar to previous work on broadcasting (in particular [15]) and gets adjusted to the different informational requirements using different schemes. The only case that gives new insights for the SINR model is (4) in Section 6, where the impossibility to access coordinates requires a more intricate strategy. Unfortunately, it is deferred almost completely to the Appendix.

Overall, the paper seems solid, but most of the approaches appear straightforward, maybe with the exception of Section 6. For the latter, the authors should elaborate on how their approach compares to the simple back-off-style algorithm from [5], which might produce a similar bound of $(n+k)\lg^i(n)$ for multi-broadcasting with much less information.

In terms of write-up, there are several problems with singular/plural, commas, and missing articles (the/a/an), especially in the introduction.

----------------------- REVIEW 2 ---------------------
----------- REVIEW -----------
In the SINR model of weak devices in the Euclidian plane the authors present deterministic distributed algorithms for the multi-broadcast of a given set of rumors. They consider four settings which differ in the presumed knowledge of the coordinates of the nodes.

The paper is nicely structured and the different settings which are considered are clearly distinguished and explained quite well (though it would have been nice to actually mention somewhere that, in the centralized setting, the IDs of all nodes are known to each node). The authors explain what the algorithms are to accomplish but there are parts of the algorithms where the correctness is not evident and no proof of correctness is given. The algorithms themselves are not always presented in a clear-cut way, the phrasing (in both algorithms and explanations) is sometimes ambiguous (for an example, see below).

The notation is not consistent throughout the paper, e.g., the set DIR resurfaces as DDL (without any explanation or definition), strongly-selective families are denoted by (X,y)-ssf (in the definition) and SSF(X,y) (if the latter should denote a certain kind of strongly-selective family, it is at least not mentioned anywhere), the number k resurfaces repeatedly as K. The readability is further diminished by several misleading mistakes like O(k log n) (instead of $O(k log \Delta)$) and parent(u)=v (instead of parent(v)=u) in Section 3.1.3.

Large parts of Section 2 are taken from [15] almost verbatim without mentioning it. While not applied to the specific problem/settings of the paper at hand before, quite a few of the employed techniques and ideas are known from previous work.

The related work section is very weak, and I believe that this paper should be rejected based on this fact already. There are several results that should be mentioned in this paper, for instance not a single result by Halldorsson (who solved various related problems in the past few years, together with a different set of co-authors) is cited.

In several places some additional details would have greatly enhanced a quicker understanding of the presented material, especially regarding references to other papers, e.g., the phrase "using the observation made in [15]" in Section 3.1.1 makes it difficult for the reader to locate the mentioned observation quickly.

For (exemplary) details regarding some of the above points consider, e.g., Section 3.1.3:
Aside from minor things (like the syntactic mistake in line 2, the double checking if state(v)=active, the ambiguous phrasing in line 6), in Protocol 2 it is not clear why there cannot be nodes which become inactive before they send any message. Furthermore there is no explanation why it is impossible that a node has more than one parent.

In Protocol 3 $l(K_C)$ (appearing as $l(T_C))$ gathers the rumors of the nodes in C, but (amongst others) Prop. 4 suggests that the gathering is done by $l(C)$.

----------------------- REVIEW 3 ---------------------
----------- REVIEW -----------
OVERVIEW

This paper studies the problem of distributed broadcast of k messages to a wireless network, under the assumption of non-spontaneous activation; i.e., non-message source nodes must receive a message before they activate and can transmit.

The paper uses an SINR model to determine message communication behavior and studies only deterministic solutions. It presents a collection of new upper bound results that combine existing techniques with new techniques to solve this problem under different assumptions concerning the knowledge.

In the following, we use n as the message size, and $\Delta$ and D to refer to the maximum degree and diameter, respectively, of the "reachability" graph formed when we add edges between nodes that can communicate with each other.

Known for single message distributed broadcast in SINR models:

1. When all nodes (not just the message sources) are activated in the first round, a backbone can be constructed by a deterministic algorithm in $O(\Delta\lg^i{n})$ rounds [11]. In [11], the authors show how to then use the back bone to solve k-message broadcast (the paper studied here) in $O(D + k + \Delta\lg^i{n})$ rounds. The results in [11] assume the same "weak device" model studied in this paper.

(As an aside, I find it unusual that the authors would cite their former result from [11] on the backbone but not mention that [11] has a result for the exact k-message problem studied here?)

2. For the case of non-spontaneous wake-up, the results in [15] show how to solve single message broadcast (k=1) in $O(n\log{n})$ rounds if nodes only know their own coordinates and $O(D\log^2{n})$ time if the also know their neighbors coordinates.

This paper asks what happens if we have k messages instead of just 1 and we consider the trickier non-spontaneous wake-up case. They offer several new upper bound results, each for a different set of assumptions on network knowledge.

Result number-1: $O(D + k\log{\Delta})$ for "centralized" algorithms.

"Centralized" seems to be used in a non-standard way. In the context of radio network broadcast, a centralized algorithm usually means that an algorithm is given a description of a network and must efficiently generate a broadcast schedule that solves the relevant broadcast problem. The setting considered in this first result seems to be different. It seems they are instead considering the case where a *distributed* algorithm is provided full network knowledge as input (i.e., all nodes know the identity and positions of all nodes) but *not* provided knowledge of the message sources. I assume this hybrid case is motivated by the setting where a network is configured carefully, then needs to dynamically execute broadcast as message arrive.

In this setting, nodes can precompute a backbone structure so the main challenge is gathering the k messages into this structure for efficient dissemination. They also show how to replace $k*\log{\Delta} with k + \lg{g}$ for granularity g (granularity captures the ratio between the maximum and minimum link in the network). When g is small, more spatial reuse is possible and the problem can be solved faster.

Result number-2: $O(D\lg^2{n} + k\lg{\Delta})$ for the case where nodes know their neighbors coordinates

The difficulty in this case is that nodes can no longer pre-compute a backbone structure. To overcome this challenge they use the same strategy form their earlier work on single message broadcast under similar assumptions [15] and combine it with strategies for the previous centralized setting.

Result number-3: $O((n+k)\lg{n})$ rounds for the case where nodes only know their own coordinates.

The core of the algorithm in this case an interesting "local learning" protocol that allows nodes to learn their neighbors (and their coordinates) in $O(n\log{n})$ time. At this point, they can use the techniques from the previous case. A similar local learning type subroutine shows up in [11], so it would be nice to hear about how these two routines differ.

Result number-4: $O((n+k)\lg{n})$ rounds for the case where all you know are the ids of your neighbors

The details of how this algorithm works and its analysis are in the paper's appendix. At a high-level, the strategy here seems to depend on message sources creating tokens which compete in the network. Ultimately, one token survives and can build a BFS tree on which efficient communication can be coordinated.

I am wondering why this result does not subsume result number-3, as the setting seems harder and the time complexity is the same?

EVALUATION

Let me first address the model (with the caveat that I very well might be mis-understanding something in my below assessment)...

The weak device model in this paper is debatable. It says that v receives a message from u if and only if two things are true: the SINR is at least $\beta$ at v for u's transmission; and the SINR would be at least $(1+\epsilon)\beta$ at v if u broadcast alone. Having a $(1+\epsilon)$ in addition to $\beta$ seems redundant. The whole purpose of $\beta$ is to capture how much more powerful than noise/interference a signal must be in order to be successfully received. Why would this threshold change depending on the composition of the interference (i.e., the reception threshold is larger than $\beta$ if the interference comes just from the N factor of the SINR equation, but can be right at $\beta$ if the interference includes noise from other transmitters in the network)?

Even if we accept the model as a theoretical variation, why is it useful? My hypothesis is that the weak model is useful for backbone algorithms because it eliminates one of the hard problems of creating backbones in the SINR model: making sure you are covered by a strong neighbor.

In more detail, the main hurdle faced by other backbone SINR papers is that it is possible that you end up covered by a backbone node only weakly connected to you. This backbone is not necessarily useful because it would not admit a lot of spatial reuse (to hear from this backbone node, you cannot tolerate much other simultaneous transmissions in the network). Whereas other papers relied on things like carefully tuned carrier sensing or power control to overcome this problem, the weak device model seems to solve it deus ex machina style by simply forbidding nodes from receiving messages from weak neighbors.

On the other hand, model justification should *not* be considered a crucial criteria in evaluating theory results, as interesting theory is interesting theory. Furthermore, it seems to me that for all but the final case they consider (Result number-4 in my above overview) you do not really need the weak device assumption as nodes have coordinates (and know the SINR equation) so they can simply label messages with their location, and receivers can simulate the weak model by throwing out messages from weak connections. It's possible I'm missing something, but if that's true, that strengthens the results and the authors should certainly emphasize where they do and do not need the extra weak assumptions.

What I liked about the paper were the routines used to gather information into the backbone, and the interesting competing-token tree-building routine of Result number-4. To the best of my knowledge, these are novel and contained some nice ideas potentially useful in other problems.

A lot of the rest of the paper, however, seemed to be building somewhat incrementally on the work of [11,15] to extend those techniques to work for multiple messages. That is, the main ideas and subroutines of [11,15] were re-used in Results 1 - 3 to get the k-message outcome.

A final minor note: the presentation needs some cleaning and can feel hastily compiled in many places. For example, the main theorems use different terms for the problem (both multi-cast [which has a specific meaning in networking different than what is studied here] and multi-broadcast], and do not include the specific network knowledge assumptions to which they apply (i.e., they main theorems do not standalone, they have to be read in the context of the
containing section to understand the results). The section headers used varying title capitalization. etc.

----------------------- REVIEW 4 ---------------------
----------- REVIEW -----------
This paper adds to the recent body of literature on broadcasting
problem in the SINR model. There are numerous settings, parameters or
assumptions that can be set; the current paper deals specifically
with: deterministic algorithms, a multi-broadcast problem, uniform
power, non-spontaneous wake-up, and no carrier sense. Additionally, a
"weak model" is assumed (see later). Finally, four different versions
are treated, depending on knowledge available to the nodes:
coordinates of everyone, of itself and its neighbors, or itself only;
or only the labels of all the neighbors.

The results given are all novel and non-trivial, some using clever
combination of known techniques, and others requiring new ideas.

The paper has, however, three main weaknesses that imply that it is
unlikely to pass the grade for acceptance at SPAA:

1) The weak model assumed here is debatable. It's main effect is to
make the problems easier to solve; specifically, it greatly simplifies
the formation of a dependable dominating set, which is the key
component in a backbone construction. The model seems to have been
invented by the authors and their collaborators, without a strong case
being made.  The claimed motivation, that the radio will not turn on
unless the signal is strong enough, implies that a form of carrier
sense / signal-strength measurement capability is available, which
conflicts with the stated assumptions.

2) The multi-broadcast problem is known to be efficiently doable given
some sets of assumptions. In particular, Yu et al. (SIROCCO 2012) gave
an algorithm that performs a multi-broadcast in time O(D + k + log n),
which is best possible. For some reason, this paper is not even
mentioned.  The assumptions made there are in some sense stronger and
in some sense weaker than the assumptions of the current paper.

  In particular, the (multi-)broadcast problem can be solved
efficiently if one can find a sparse set of nodes that robustly
dominate the whole (by sparse, we mean any neighborhood contains only
a constant number of dominators; by robust, we mean that there be no
weak communication links used, which is automatically avoided in this
weak model). This can be achieved using certain assumptions
(randomization, power control, carrier sense) that do hold for even
cheap wireless gadgets today. The assumptions used here are not
particularly convincing: in order to obtain O(D polylog(n))
complexity, the nodes seem to need to know the coordinates of all their
neighbors.

 The point is that the authors fail to extract the lessons that can be
learned from their results. Yes, the particular set of assumptions
they make result in particular complexity results, but what does that
tell us that is of intrinsic interest?  Especially given the
combinatorial explosion in the number of possible sets of assumptions.

3) Finally, the discussion of related work, and the essential
comparisons and contrasts, leave much to be desired. The work of the
authors is treated in considerable detail, including their work on the
radio network model.  Work on other problems (than broadcast) in the
SINR model is just said to be "vast" and the reader simply directed to a
four-year old survey.  At the very least, this discussion of related
results is surprisingly self-centered.

What is more problematic, however, is that the work of others on
broadcast problems in the SINR model (the ones that are actually
cited) is summarily dismissed as "other [solutions] in slightly
different models". This means that there is no compare or contrast, or
any attempt to place the authors' work in a proper context. The result
is that the burden is placed on the reader (and the reviewers...) to
figure out what is truly novel with the results given and what is of
particular interest.
